# Supplementary material for: Decentralized Structural-RNN for Robot Crowd Navigation with Deep Reinforcement Learning
Source: arXiv:2011.04820 source file (2025-01-27)
Supplement: Supplementary file 1 [file Appendix.tex]

\section{Appendix}
\label{sec:append}
Not provided in the submitted version
